# Supplementary material for: A Computational-Graph Partitioning Method for Training Memory-Constrained DNNs
Source: arXiv:2008.08636 source file (2021-05-05)
Supplement: Supplementary file 1 [file appendix.tex]

\subsection{Time Complexity of Each Step of \algo{}}

{\bf Complexity of Graph Slicing:} The most expensive part of Algorithm~\ref{alg1} is computing weighted levels for all the nodes. 
This operation performs a variant of topological sorting and has time complexity of ${O(\vert V \vert + \vert E \vert)}$~\cite{sinnen2007task}. It is done $K$ times, resulting in an overall complexity of ${O(K(\vert V \vert + \vert E \vert))}$ as opposed to linear clustering that would cost ${O(\vert V \vert(\vert E \vert + \vert V \vert))}$~\cite{wang2018list}.
%, resulting in a lot more expensive slicing than ours. 
%yields relatively low quality~\cite{wang2018list}. 

{\bf Complexity of Mapping:} Since the clusters are disjoint paths or singular nodes, and have no common nodes (a node exists only in one cluster), the total number of  the update operations is bounded by ${\vert V \vert}$. The number of range summation queries is bounded by the number of the paths which is again bounded by ${\vert V \vert}$. The cost of either of the operations is logarithmic in the number of levels. The number of levels is ${\leq \vert V \vert}$, so we end up with ${O(\vert V \vert * log\vert V \vert)}$. Before starting LALB, we sort the clusters by their weights (the heaviest clusters first due to their importance in balancing the loads), this has an upper bound of ${O(\vert V \vert * log\vert V \vert)}$, since the number of clusters is upper-bounded by the number of nodes. Hence, the overall complexity of the mapping stage is ${O(\vert V \vert * log\vert V \vert)}$.

{\bf Complexity of Refinement:} For swapping, initially we sort the clusters by ${tl(n)}$ of their source nodes to find the clusters within the span of a certain cluster using binary search. Since the number of disjoint clusters is bounded by the number of nodes, this process 
gives the complexity of ${O(\vert V \vert*log(\vert V \vert))}$.  Once two clusters are swapped, they are marked and not considered again leading to at most $\vert V \vert$ cluster, hence node, swaps. With each swap the binary-indexed-trees are updated to reflect the new work loads. Since each update takes ${O(log(\vert V \vert))},$ overall complexity is ${O(\vert V \vert*log(\vert V \vert))}$. The node-level refinement is repeated ${K}$ times and each time we recalculate the weighted levels and the $CP$. Upon node switching we update the trees. The overall time complexity is ${O(K(\vert V \vert + \vert E \vert))}$.

{\bf Complexity of Scheduler Emulator:} The scheduler emulator estimates the starting time ${st(n)}$ and finishing time ${ft(n)}$ of the nodes in the graph. The emulator has time complexity of ${O(\vert V \vert+ \vert E \vert)}$.

{\bf Complexity of Tracking Memory Consumption:} Tracking the memory consumption requires ${O(\vert V \vert)}$ time since it is done in one pass over the graph nodes while keeping the cumulative values and calculating the potentials.

 {\bf Complexity of Addressing Overflow:} We solve the knapsack greedily as the dynamic programming based solution complexity is impractical. When an overflow is detected, we pick the nodes from the heaps in a logarithmic time. 
 Any node that is moved to another partition is guaranteed not to be moved again since it is moved only if the destination $pe$ can accommodate it, meaning that it can neither cause nor solve an overflow on that $pe$. As a result, there is no repetition and a node can enter or exit the heap once, resulting in $O(\vert V \vert *log \vert V \vert)$. When a node is moved, the new potentials and memory consumption need to be recalculated (${O(\vert V \vert)}$). It may happen at most $\vert V \vert$ times. Overall the complexity is $O(\vert V \vert^2)$.
 
 \subsection{Models and Datasets}

From the language modeling, we use \textbf{Word-RNN} a multi-layer Recurrent Neural Network for word-level language inspired by the character-level modeling~\cite{sutskever2011generating}, and character-Aware Neural Language Models (\textbf{Char-CRN})~\cite{kim2016character}.
Both models can be enlarged by increasing the number of layers or the hidden state size. While Penn Treebank text corpus ~\cite{marcus1994penn} is used to train \textbf{Char-CRN}, \textbf{Word-RNN} is trained using Tiny Shakespeare~\cite{tinyshakespeare_2015}.

From computer vision, we experiment with \textbf{WRN}~\cite{zagoruyko2016wide}, which is a widened version of the residual network model. In \textbf{WRN} the width of the convolutional layers can be configured. The model size grows quadratically when widened. WRN has achieved better accuracy when the model is widened~\cite{zagoruyko2016wide}. \textbf{WRN} is trained using  \textbf{CIFAR}~\cite{krizhevsky2009learning} as it is the dataset used by the original authors. 

\textbf{TRN} (Transformer)~\cite{vaswani2017attention} 
is a widely used model that had a significant influence on the design of SoTA Transformer-based models in the NLP domain such as GPT-2~\cite{radford2019language} and Megatron-LM~\cite{shoeybi2019megatron}. 
Transformer can be enlarged by increasing the number of layers, which deepens the model, and by widening the inner-layer dimensionality.  Deeper~\cite{huang2019gpipe} and wider~\cite{vaswani2017attention} configurations of Transformer are shown to give higher accuracy. We trained Transformer using IWSLT 2016 German–English parallel corpus for training. 

\textbf{E3D} is Eidetic 3D LSTM~\cite{wang2018eidetic} for video prediction. This model achieves state-of-the-art performance in future frame prediction. {\em E3D} is closely related to convolutional recurrent networks, where the dimensions of memory states are increased, and 3D-Convs are adopted as the basic operators for state transitions. \textbf{E3D} can be enlarged by increasing the number of the hidden state channels on the memory dimensions. We trained E3D-LSTM using the Moving MNIST dataset.
